# Supplementary material for: Continuous Integration Practices in Machine Learning Projects: The Practitioners` Perspective
Source: arXiv:2502.17378 source file (2025-02-24)
Supplement: Supplementary file 1 [file appendix_tesseract-ocr_tesseract-form.pdf]

# Continuous Integration Practices in Machine Learning Projects

The adoption of a CI service such as GitHub Actions is only the first step to enforce a set of CI practices that contribute to project stability and reliability. These practices encompass ***automatically and frequently testing and integrating code changes, maintaining a higher test coverage, keeping short build duration, and quickly fixing broken builds.***

**Note:** In the context of GitHub Actions, "build" explicitly refers to a GitHub Actions CI Workflow Run.

This survey will ask 8 open-ended and 12 closed-ended questions about adopting CI practices in ML projects and will take ***less than 10 minutes to complete.*** We will also provide data derived from the [\*\*tesseract-ocr/tesseract\*\*](#) project to frame our inquiries.

This study considers ML projects as ML frameworks and libraries or ML applications that use ML-based components in their functionality. It also considers non-ML projects as traditional software applications, including web/mobile frameworks and applications, desktop applications, static site generators, cloud tools, package management, and other software projects characterized by the absence of ML-based components in both design and functionality.

**IMPORTANT:** By answering this form, you agree to use your own experience and not rely on Large Language Models (LLMs), such as ChatGPT, to generate your answers.

Please don't hesitate to contact us if you have any questions or require further clarification.

João Helis Bernardo  
Federal University of Rio Grande do Norte, Brazil  
E-mail: [joaohelis@ppgsc.ufrn.br](mailto:joaohelis@ppgsc.ufrn.br)

By completing this survey, you will be entered into a drawing to win one of ten \$50 Amazon or Steam gift cards. If you would like to participate in the drawing, please select one of the options below.

*\* Only participants who answer all questions will be eligible for the drawing.*

*Mark only one oval.*

- ☐ I want to participate in the drawing for a \$50 Amazon gift card.
- ☐ I want to participate in the drawing for a \$50 Steam gift card.

## 1. Participant Information

1.1. For how long have you been developing software?

*Mark only one oval.*

- ☐ Less than 2 years
- ☐ 2 - 4 years
- ☐ 5 - 7 years
- ☐ 8 - 10 years
- ☐ More than 10 years

1.2. For how long have you been contributing to ML projects?

*Mark only one oval.*

- ☐ Less than 2 years
- ☐ 2 - 4 years
- ☐ 5 - 7 years
- ☐ 8 - 10 years
- ☐ More than 10 years

1.3. What are your primary roles in the ML projects you contribute to? (Select all that apply)

*Check all that apply.*

- ☐ Developer
- ☐ Data Engineer [Data ingestion / Data Store]
- ☐ Data Scientist [Model development and validation]
- ☐ ML Engineer [Model deployment and monitoring]
- ☐ Reviewer/Integrator
- ☐ Tester
- ☐ DevOps Engineer
- ☐ Other: \_\_\_\_\_

1.4. How familiar are you with the concept of Continuous Integration?

*Mark only one oval.*

- ☐ Not familiar at all
- ☐ Somewhat familiar
- ☐ Moderately familiar
- ☐ Very familiar
- ☐ Extremely familiar

## 2. Perceptions about the difference in CI practices adoption between ML and non-ML projects

2.1. As an integrator of an ML project, do you believe your team strives to incorporate CI practices, such as committing changes frequently, maintaining short build durations, quickly addressing broken builds, and upholding high test coverage levels, within its workflow?

---

---

---

---

---

2.2. What unique challenges or differences exist, if any, when implementing a CI pipeline (i.e., GitHub Actions CI workflows) on ML projects compared to non-ML projects?

---

---

---

---

---

2.3. To what extent do ML projects **commit more frequently** when compared to non-ML projects?

*Mark only one oval.*

- ☐ Always
- ☐ Often
- ☐ Sometimes
- ☐ Rarely
- ☐ Never

2.4. To which frequency do ML projects have **longer build durations** when compared to non-ML projects?

*Mark only one oval.*

- ☐ Always
- ☐ Often
- ☐ Sometimes
- ☐ Rarely
- ☐ Never

2.5. To which frequency do ML projects have a **lower test coverage rate** when compared to non-ML projects?

*Mark only one oval.*

- ☐ Always
- ☐ Often
- ☐ Sometimes
- ☐ Rarely
- ☐ Never

2.6. To which frequency do ML projects **fix broken builds more quickly** when compared to non-ML projects?

*Mark only one oval.*

- ☐ Always
- ☐ Often
- ☐ Sometimes
- ☐ Rarely
- ☐ Never

### 3. Perceptions about the results of our previous study

In our previous study (available at <https://ci-ml-msr.github.io>), we examined 185 open-source projects on GitHub, comprising 93 ML projects and 92 non-ML projects. Our goal was to uncover disparities in CI adoption between ML and non-ML projects. In the following questions of this survey, we will present specific data from our study and seek your insights into the reasons behind our findings.

3.1. How important or unimportant are ML projects keeping a short build duration?

Mark only one oval.

- ☐ Not at all important
- ☐ Slightly important
- ☐ Important
- ☐ Fairly important
- ☐ Very important

3.2. According to our data, **ML projects generally have longer build durations** than non-ML projects across different project sizes. For example, small ML projects (Lines of Code [LOC]  $\leq 10,000$ ) have a median build duration of 10.3 minutes, compared to 0.8 minutes for small non-ML projects. Medium-sized ML projects ( $10,000 < \text{LOC} \leq 100,000$ ) take a median of 13 minutes, while non-ML projects take 5.5 minutes. Large ML projects ( $\text{LOC} > 100,000$ ) require a median of 21.4 minutes, compared to 17.4 minutes for large non-ML projects. Do these findings align with your expectations, and if so, why?

---

---

---

---

---

3.3. What strategies or techniques do you think ML projects could employ to reduce their build duration?

---

---

---

---

---

3.4. In your opinion, what would be an acceptable test coverage rate for an ML project?

Mark only one oval.

- ☐ (90% - 100%]
- ☐ (80% - 90%]
- ☐ (70% - 80%]
- ☐ (60% - 70%]
- ☐ (50% - 60%]
- ☐ (40% - 50%]
- ☐ (30% - 40%]
- ☐ (20% - 30%]
- ☐ (10% - 20%]
- ☐ [0% - 10%]
- ☐ It is indifferent

3.5. When analyzing the data from the studied projects, we noticed that medium-sized ML projects ( $10,000 < \text{LOC} \leq 100,000$ ) exhibit a lower test coverage rate compared to non-ML projects. Do these findings align with your expectations? If so, why do you think this discrepancy exists?

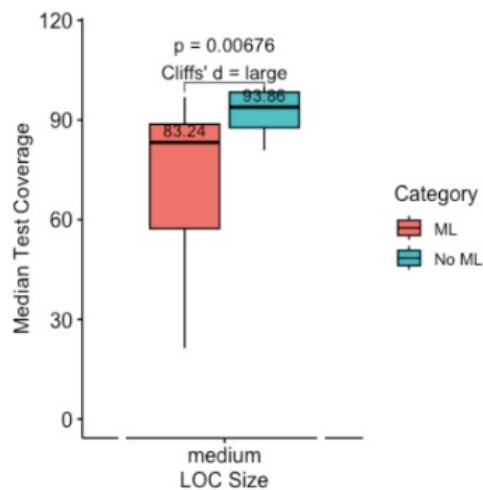

---

---

---

---

---

3.6. Can you identify any specific challenges unique to Machine Learning projects when testing their source code?

---

3.7. What strategies or techniques do you believe ML projects could implement to enhance their test coverage over time?

---

---

---

---

---

#### 4. Specific questions for the project **tesseract-ocr/tesseract**

4.1. How would you rate your familiarity with the CI pipeline employed in the **tesseract-ocr/tesseract** project?

Mark only one oval.

- ☐ Very Poor
- ☐ Poor
- ☐ Fair
- ☐ Good
- ☐ Excellent

4.2. In your opinion, what would be an acceptable build duration for a Machine Learning project of comparable size to **tesseract-ocr/tesseract**?

Mark only one oval.

- ☐ Less than 10 minutes
- ☐ 10 - 20 minutes
- ☐ 20 - 30 minutes
- ☐ 30 - 40 minutes
- ☐ 40 - 50 minutes
- ☐ 50 - 60 minutes
- ☐ More than 60 minutes
- ☐ It is indifferent

4.3. When analyzing the data of the **tesseract-ocr/tesseract** project, we observed that this project has a median build duration of **124.9 minutes**, which is **longer than 90% of the investigated projects** of similar size. Do you have any insights into why this project has a longer build duration?

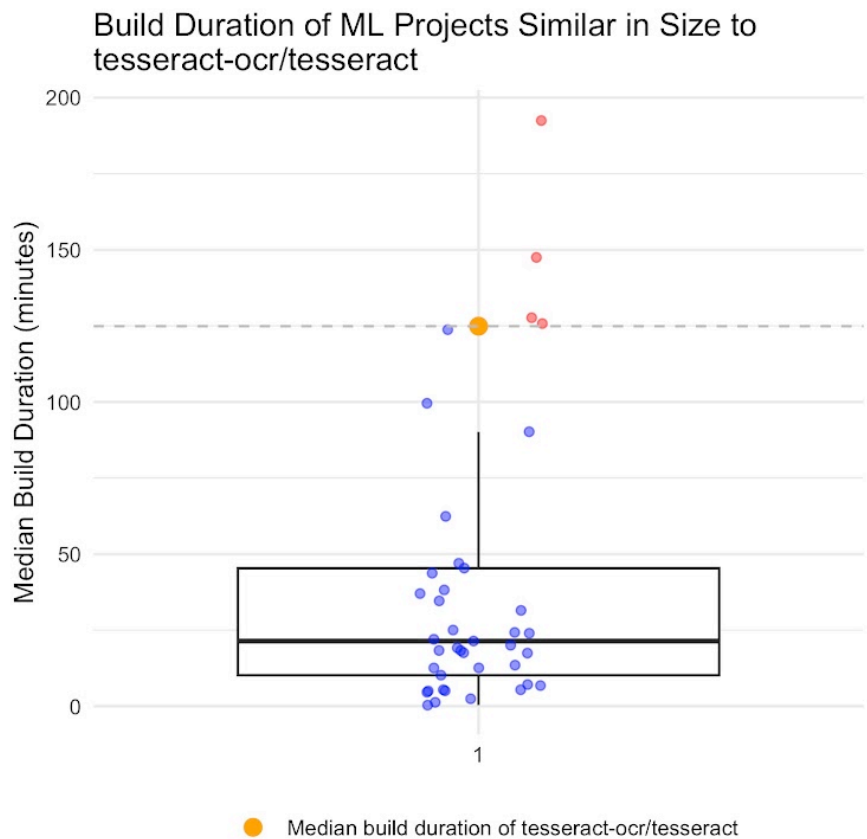

---

---

---

---

---

5. Ending our questionnaire

5.1. Would you like to be informed about our findings?

*Mark only one oval.*

☐ Yes

☐ No

5.2. Would you be willing to be contacted for a quick online follow-up interview (at a time convenient for you)?

*Mark only one oval.*

☐ Yes

☐ No

5.3. If you answered "yes" to either of the two questions above or indicated at the beginning of the form that you want to participate in the gift card drawing, please provide your email address below.

---

5.4. Do you have further comments for us?

---

---

---

---

---

---

This content is neither created nor endorsed by Google.

Google Forms
